# Supplementary material for: Live Functional Programming with Typed Holes
Source: arXiv:1805.00155 source file (2018-11-20)
Supplement: Supplementary file 1 [file implementation-appendix.tex]

% !TEX root = hazelnut-dynamics.tex

\section{Implementation Screenshots}
\label{sec:impl-screenshots}

\begin{figure}[h]
\includegraphics[width=\textwidth]{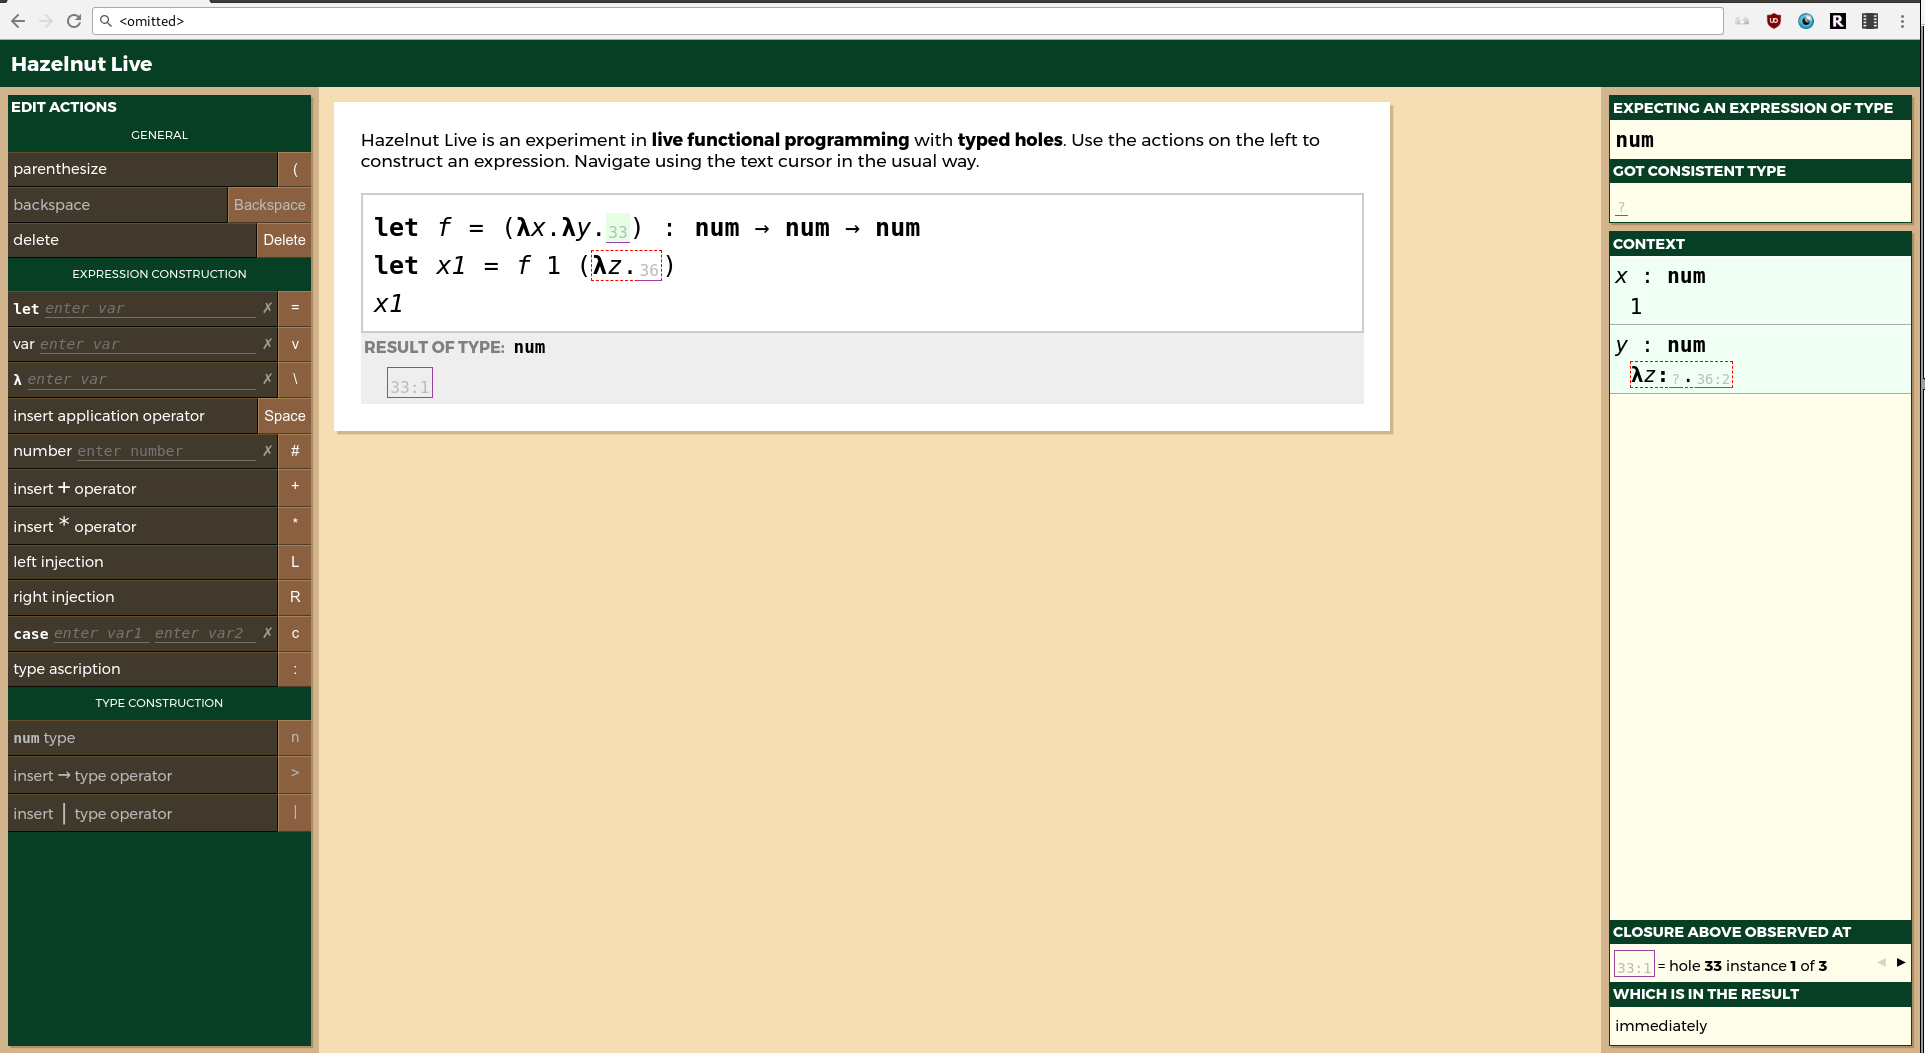}
\caption{This screenshot demonstrates both empty and non-empty expression holes as well as the live context inspector.}
\end{figure}

\begin{figure}[h]
\includegraphics[width=\textwidth]{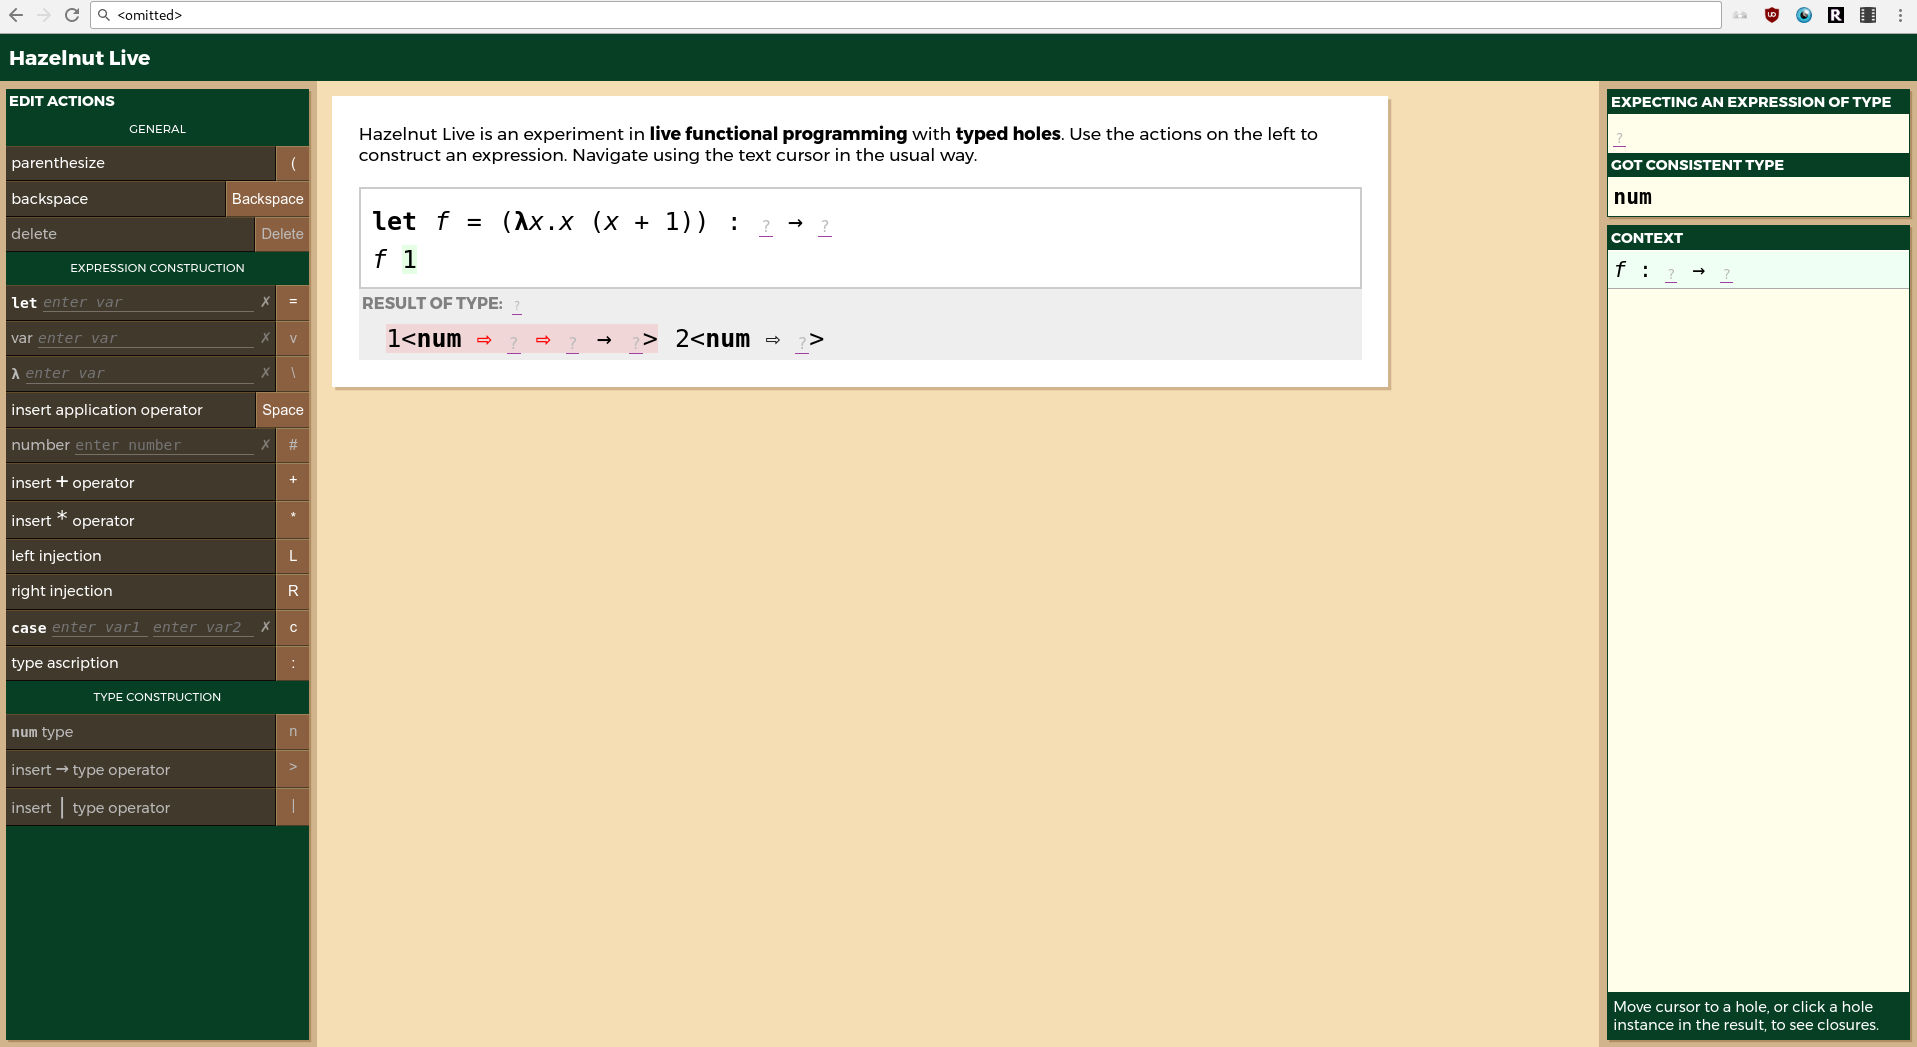}
\caption{This screenshot demonstrates dynamic cast failure.}
\end{figure}
